# Supplementary material for: Prompt Augmentation for Self-supervised Text-guided Image Manipulation
Source: arXiv:2412.13081 source file (2024-12-17)
Supplement: Supplementary file 1 [file X_suppl.tex]

\clearpage
\setcounter{page}{1}
\setcounter{figure}{0}
\setcounter{table}{0}
\setcounter{section}{0}

\maketitlesupplementary

In this supplementary material, we delve deeper into the capabilities of our proposed method for text-guided image manipulation. Included are implementation details, limitations, illustrative samples of prompt augmentations, insights into the mask generation process, and supplementary qualitative comparisons that further enrich the findings presented in the main paper.

\section{Implementation Details} We employed a pretrained LDM, specifically Stable Diffusion v1.4, as the foundation of our experiments. Fine-tuning the UNet was conducted for 20,000 steps, utilising a learning rate of 1.0e-05. The experiments were executed on an NVIDIA Titan RTX with 24GB of GPU memory, employing a batch size of 1. The image size used was 384, and we augmented each image with 3 target prompts as decsribed in Sec.~\ref{sec:prompt_augmentation}.

\section{Limitations}

While our work demonstrates notable achievements in image manipulation, it is crucial to acknowledge its limitations.
Prompt augmentation, while beneficial for introducing diversity during training, presents challenges. Overreliance on augmented prompts may carry the risk of bias, potentially hindering the model's generalisation to new prompts. Our current strategy, focusing on the manipulation of adjectives and nouns, represents a subset of the infinite possibilities for image edits. Hence, the augmentation process remains suboptimal, emphasising the need for more sophisticated techniques, potentially involving the training of a dedicated large language model for this purpose. Additionally, the resource limitations with a batch size of 1 limits the potential of our approach.

\section{Prompt Augmentation and Mask Generation}

\begin{table}[t]
    \centering
    \resizebox{\linewidth}{!}{
    \begin{tabular}{ccc}
        \toprule
        \textbf{Input} & \textbf{Augmented Prompts} & \textbf{Generated Mask} \\
        \midrule
        \begin{tabular}{c}
            \includegraphics[width=3cm]{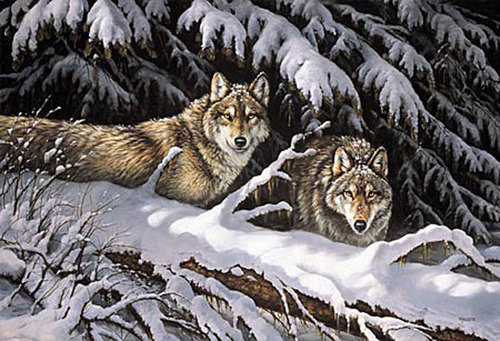} \\
            \emph{Two wolves in the snow}
        \end{tabular}
        & 
        \begin{tabular}{c}
            Two \textit{werewolves} in the snow\\
            Two \textit{cats} in the snow\\
            Two \textit{trees} in the snow\\
        \end{tabular}
        & 
        \begin{tabular}{c}
            \includegraphics[width=3cm]{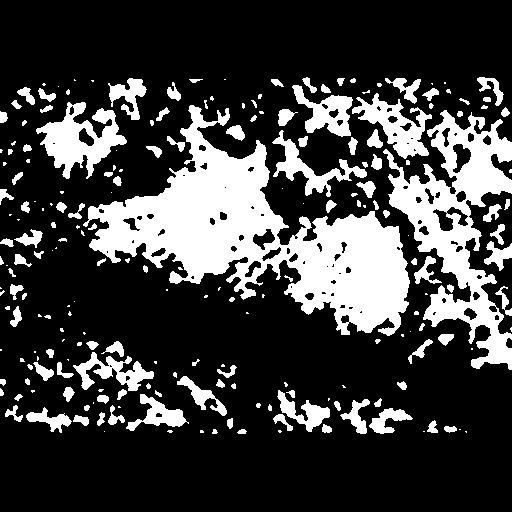}
            \\ 
        \end{tabular} \\
        \midrule
        \begin{tabular}{c}
            \includegraphics[width=3cm]{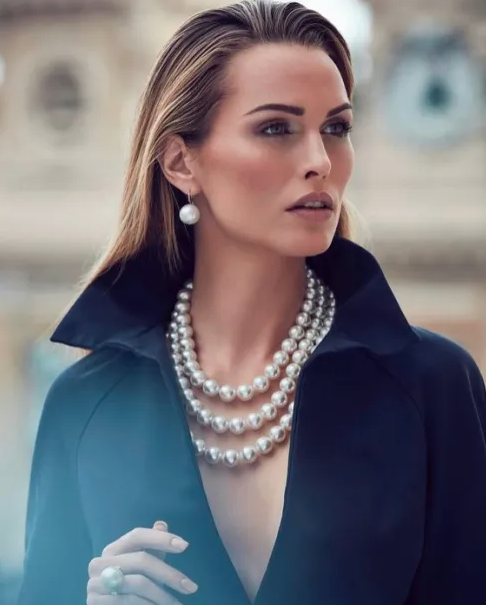} \\
            \emph{A woman wearing a pearl  necklace}
        \end{tabular}
        & 
        \begin{tabular}{c}
            A woman wearing a \textit{silver} necklace\\
            A woman wearing a \textit{sapphire} necklace\\
            A woman wearing a \textit{charm} necklace\\
        \end{tabular}
        & 
        \begin{tabular}{c}
            \includegraphics[width=3cm]{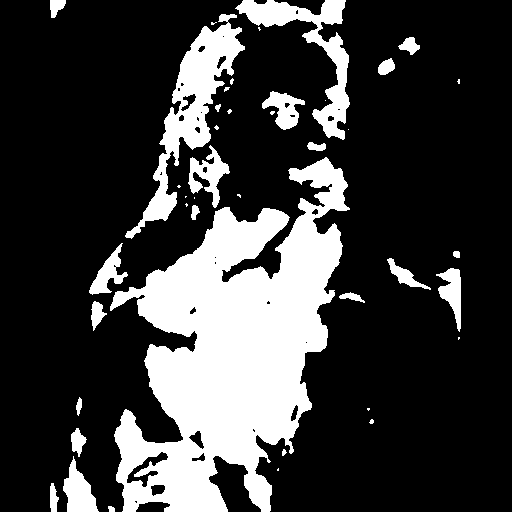}
        \end{tabular} \\
        \midrule
        \begin{tabular}{c}
            \includegraphics[width=3cm]{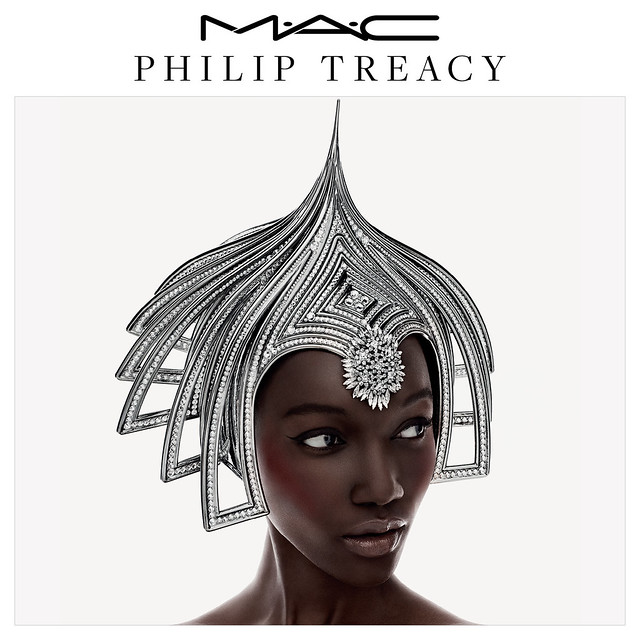} \\
            \emph{A woman wearing a silver  headpiece}
        \end{tabular}
        & 
        \begin{tabular}{c}
            A woman wearing a \textit{silvery} headpiece\\
            A woman wearing a \textit{sterling} headpiece\\
            A woman wearing a \textit{jade} headpiece\\
        \end{tabular}
        & 
        \begin{tabular}{c}
            \includegraphics[width=3cm]{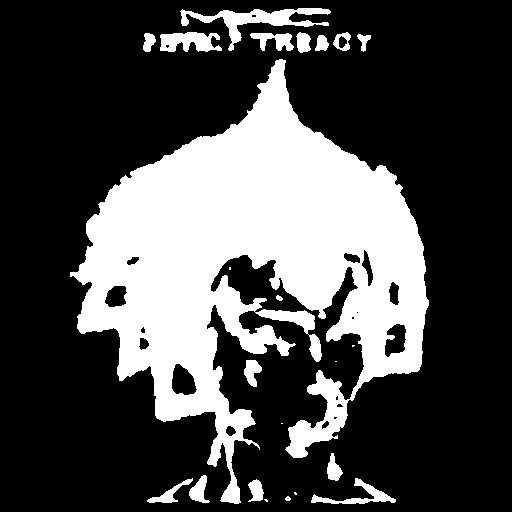}
        \end{tabular} \\
        \midrule
        \begin{tabular}{c}
            \includegraphics[width=3cm]{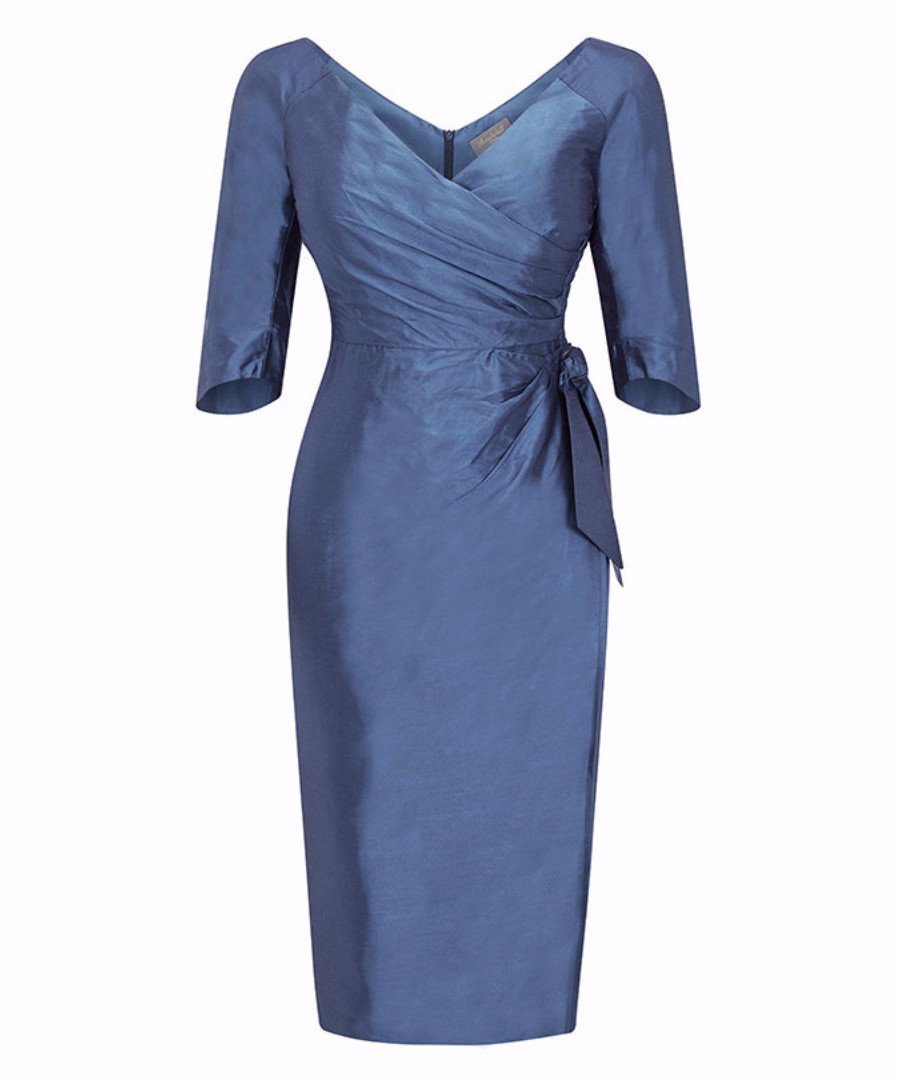} \\
            \emph{A blue dress}
        \end{tabular}
        & 
        \begin{tabular}{c}
            A \textit{black} dress\\
            A \textit{white} dress\\
            A \textit{red} dress\\
        \end{tabular}
        & 
        \begin{tabular}{c}
            \includegraphics[width=3cm]{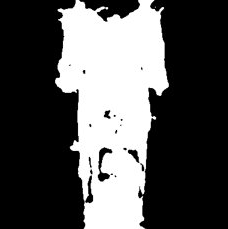}
        \end{tabular} \\
        \midrule
        \begin{tabular}{c}
            \includegraphics[width=3cm]{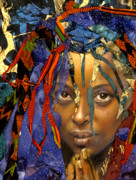} \\
            \emph{A woman with blue hair}
        \end{tabular}
        & 
        \begin{tabular}{c}
            A woman with \textit{black} hair\\
            A woman with \textit{green} hair\\
            A woman with \textit{red} hair\\
        \end{tabular}
        & 
        \begin{tabular}{c}
            \includegraphics[width=3cm]{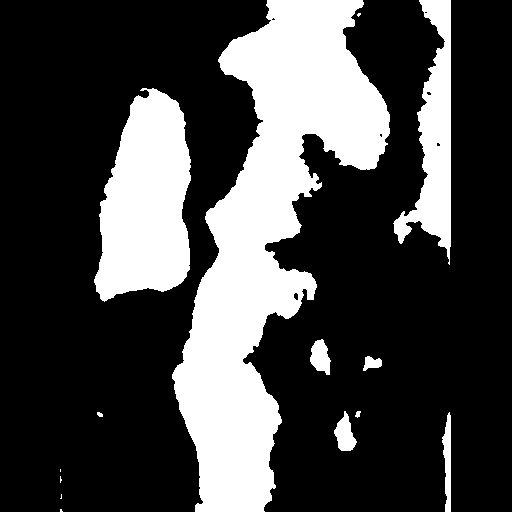}
        \end{tabular} \\

        \midrule
        \begin{tabular}{c}
            \includegraphics[width=3cm]{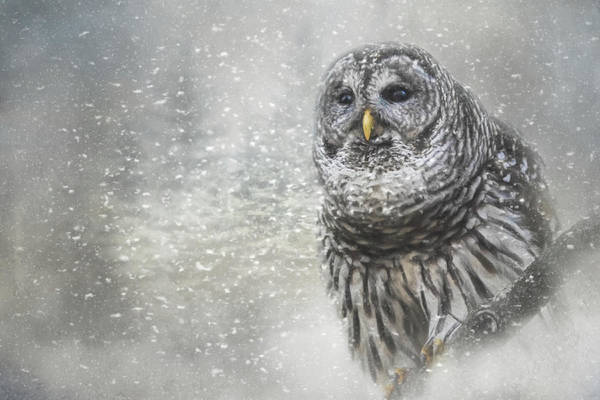} \\
            \emph{An owl in the snow}
        \end{tabular}
        & 
        \begin{tabular}{c}
            An \textit{eagle} in the snow\\
            A \textit{goose} in the snow\\
            An \textit{elf} in the snow\\
        \end{tabular}
        & 
        \begin{tabular}{c}
            \includegraphics[width=3cm]{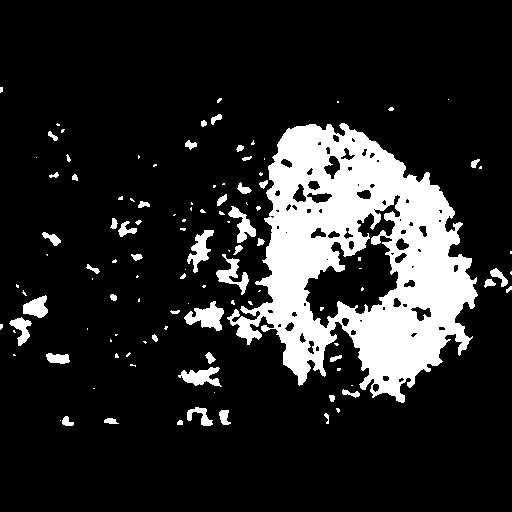}
        \end{tabular} \\

        \midrule
        \begin{tabular}{c}
            \includegraphics[width=3cm]{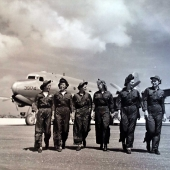} \\
            \emph{A group of men standing in front of an airplane}
        \end{tabular}
        & 
        \begin{tabular}{c}
            A group of \textit{gentlemen} standing in front of an airplane\\
            A group of \textit{monks} standing in front of an airplane\\
            A group of \textit{pirates} standing in front of an airplane\\
        \end{tabular}
        & 
        \begin{tabular}{c}
            \includegraphics[width=3cm]{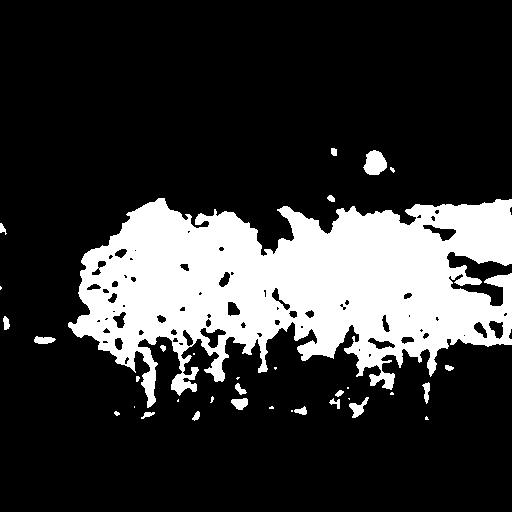}
        \end{tabular} \\

        \midrule
        \begin{tabular}{c}
            \includegraphics[width=3cm]{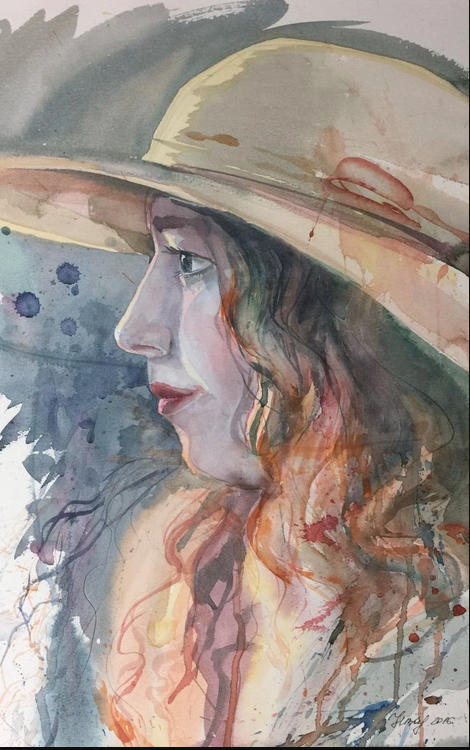} \\
            \emph{A woman wearing a hat}
        \end{tabular}
        & 
        \begin{tabular}{c}
            A woman wearing a \textit{cap}\\
            A woman wearing a \textit{hood}\\
            A woman wearing a \textit{cloak}\\
        \end{tabular}
        & 
        \begin{tabular}{c}
            \includegraphics[width=3cm]{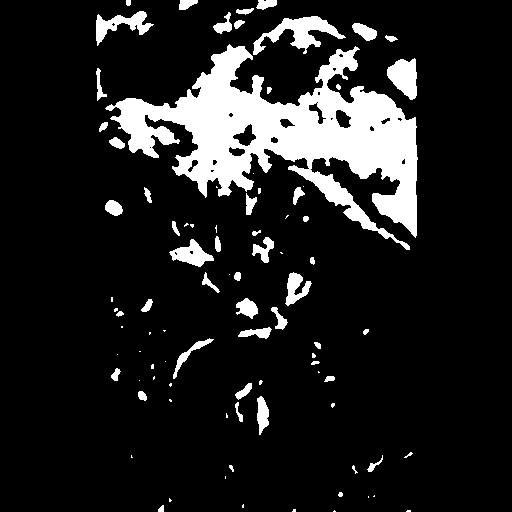}
        \end{tabular} \\
        \bottomrule
    \end{tabular}}
    \caption{Samples for prompt augmentation and the masks generated by using these prompts.}
    \label{tab:yourlabel}
\end{table}

In Figure \ref{tab:yourlabel}, we present a set of samples illustrating the augmentation process and mask generation. The "Input" column features images dynamically captioned by using BLIP~\cite{li2022blip}, offering diverse scenes.
The ``Augmented Prompts" column displays variations for each input, providing insights into augmentation diversity. For example, for an image with wolves, augmented prompts include ``Two werewolves in the snow," ``Two cats in the snow," and ``Two trees in the snow." These variations serve the purpose of the proposed soft contrastive loss.
In the ``Generated Mask" column, masks are featured, generated by leveraging the augmented prompts. The alignment of images and masks in the table provides a clear view of the augmentation and mask generation results.

\section{Additional Qualitative Comparisons}

\begin{figure*}
  \centering
  \resizebox{0.9\textwidth}{!}{%
    \begin{tabular}{ccccccc}
      input &  & SDEdit & DALL-E 2 & DiffEdit & InstructPix2Pix  & Ours \\

      \includegraphics[width=3cm]{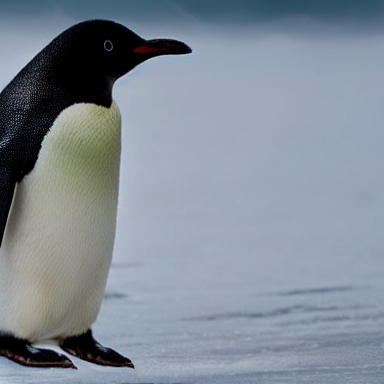} & \raisebox{0.5cm}{\rotatebox{90}{\parbox{2cm}{\centering a penguin walking on the \cancel{ice} \textcolor{red}{beach}}}} & \includegraphics[width=3cm]{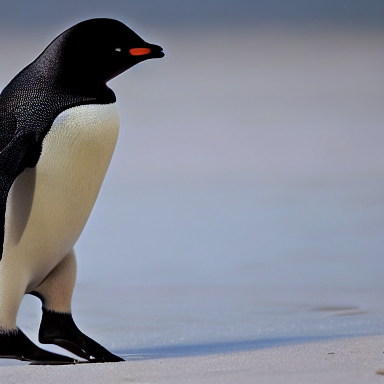} & \includegraphics[width=3cm]{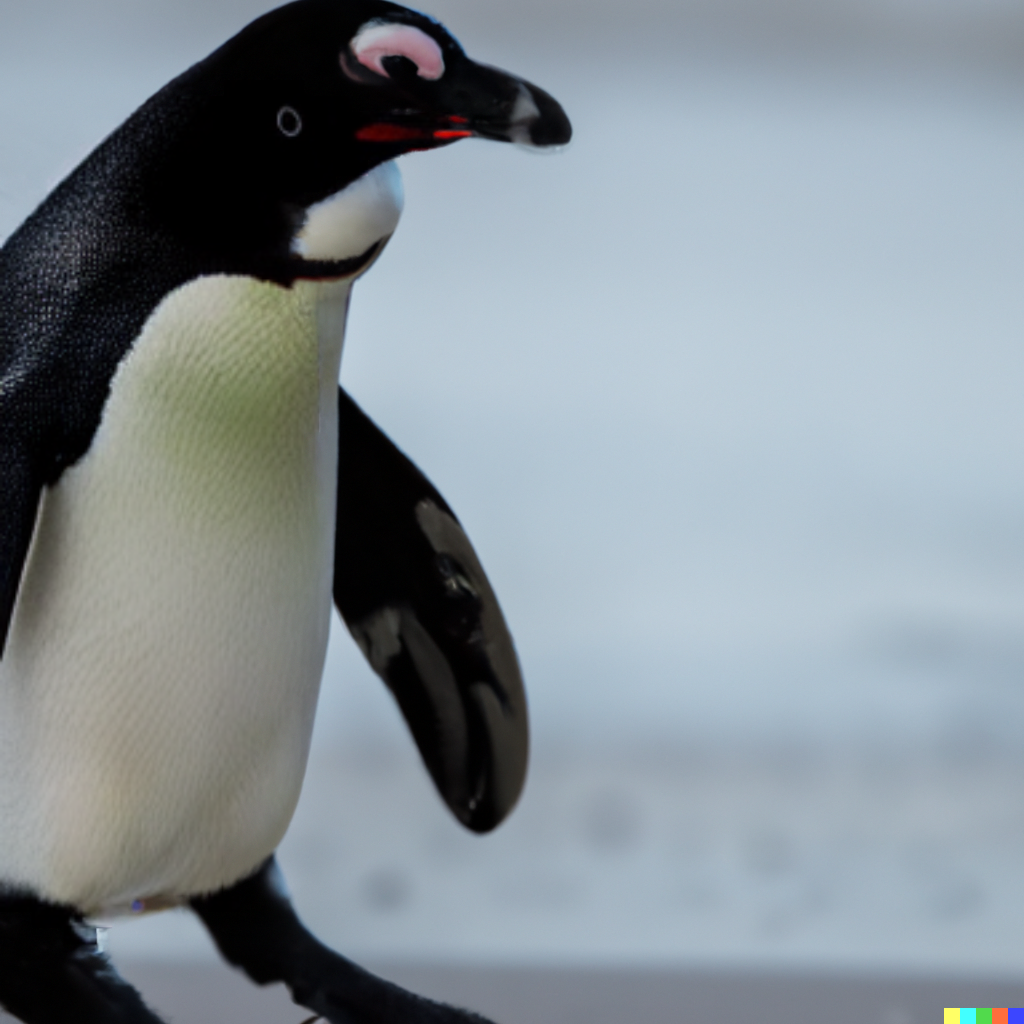} & \includegraphics[width=3cm]{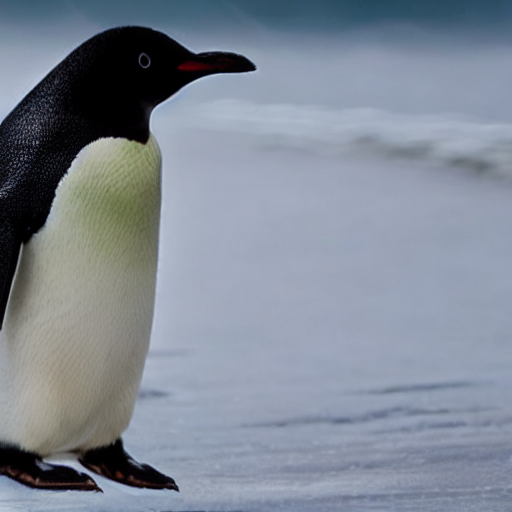} & \includegraphics[width=3cm]{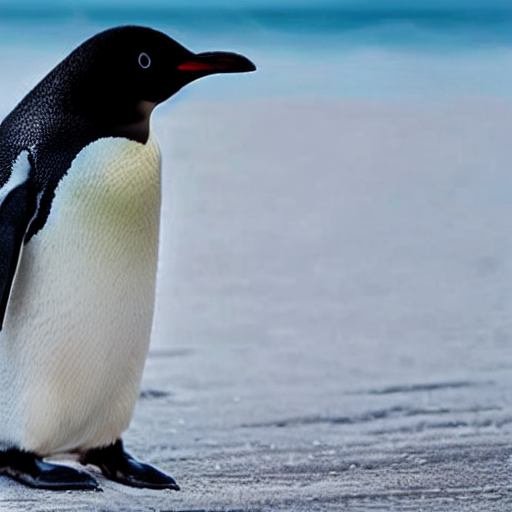} & \includegraphics[width=3cm]{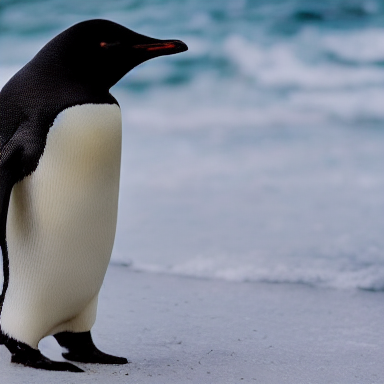}\\

      \includegraphics[width=3cm]{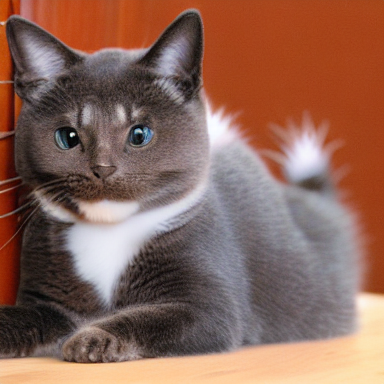} & \raisebox{0.5cm}{\rotatebox{90}{\parbox{2cm}{\centering a \cancel{cat}\textcolor{red}{leopard}}}} & \includegraphics[width=3cm]{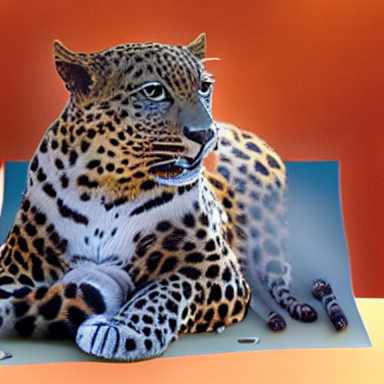} & \includegraphics[width=3cm]{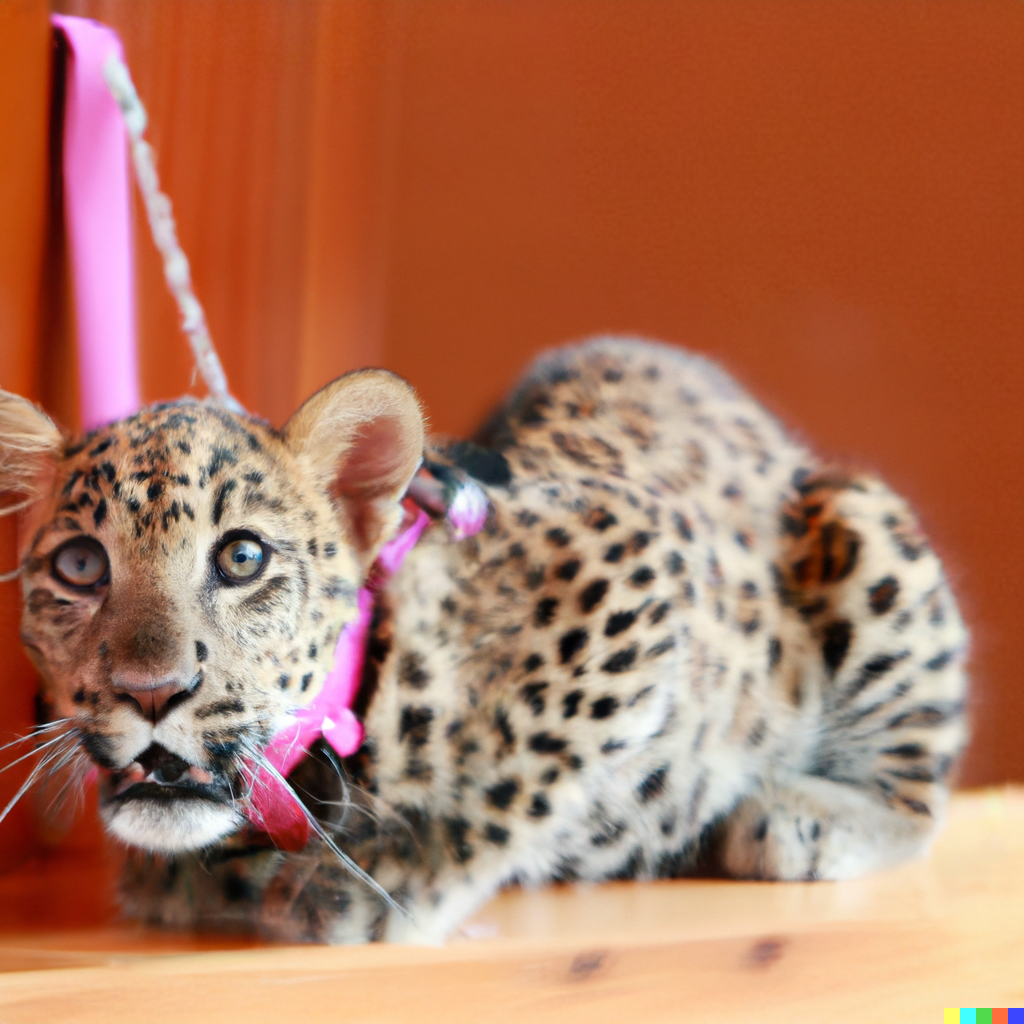} & \includegraphics[width=3cm]{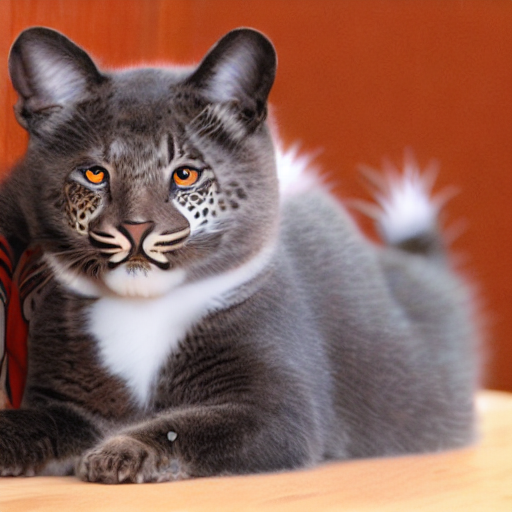} & \includegraphics[width=3cm]{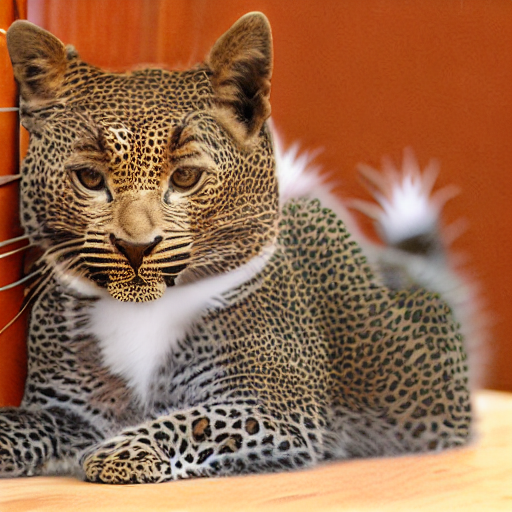} & \includegraphics[width=3cm]{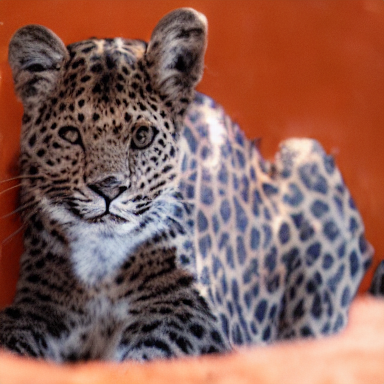}\\

      \includegraphics[width=3cm]{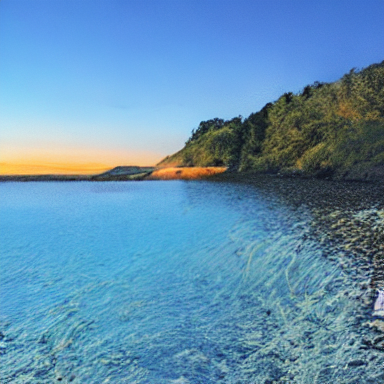} & \raisebox{0.5cm}{\rotatebox{90}{\parbox{2cm}{\centering a \textcolor{red}{boat} in the sea}}} & \includegraphics[width=3cm]{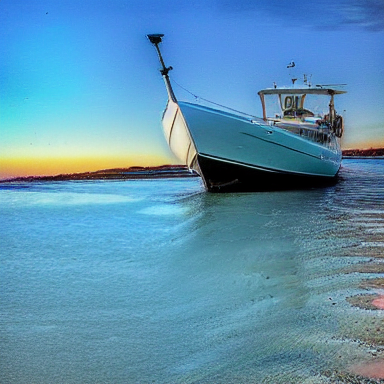} & \includegraphics[width=3cm]{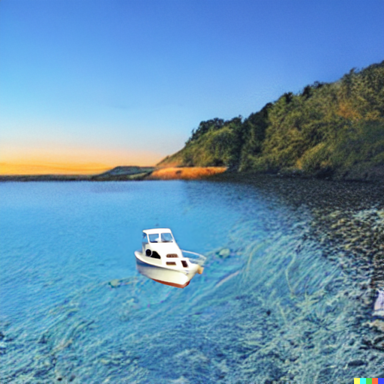} & \includegraphics[width=3cm]{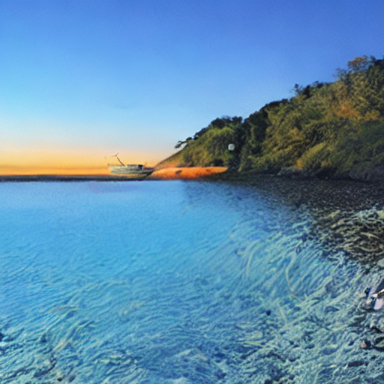} & \includegraphics[width=3cm]{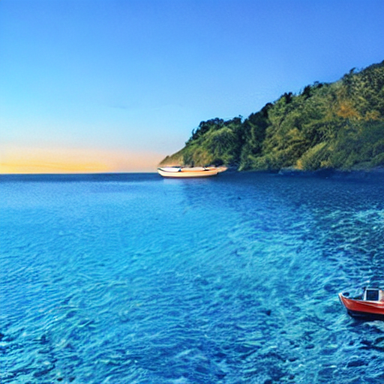} & \includegraphics[width=3cm]{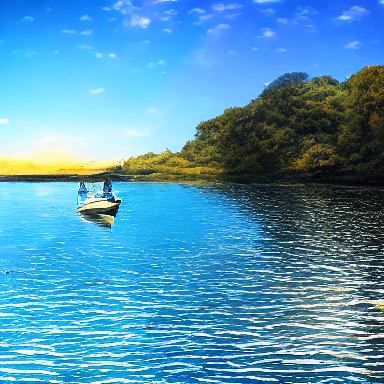}\\

      \includegraphics[width=3cm]{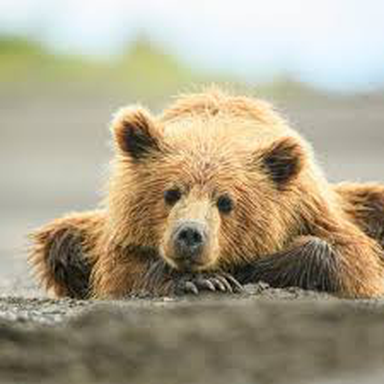} & \raisebox{0.5cm}{\rotatebox{90}{\parbox{2cm}{\centering a \textcolor{red}{panda}}}} & \includegraphics[width=3cm]{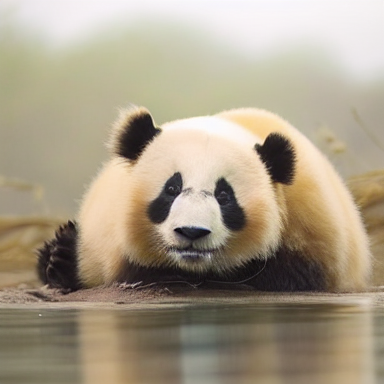} & \includegraphics[width=3cm]{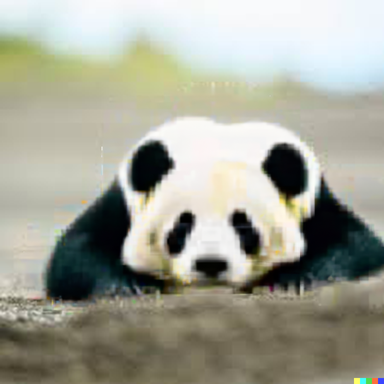} & \includegraphics[width=3cm]{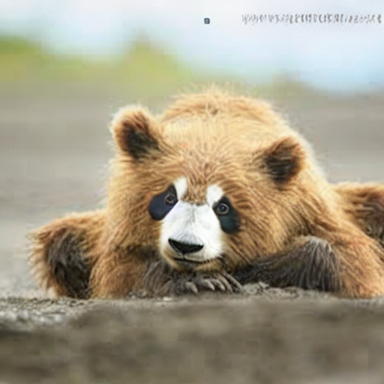} & \includegraphics[width=3cm]{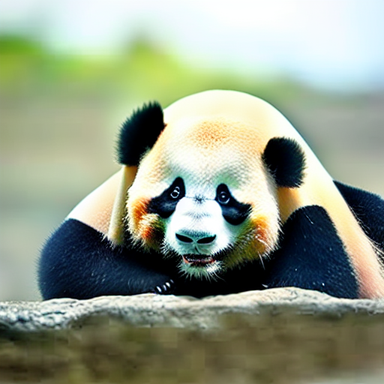} & \includegraphics[width=3cm]{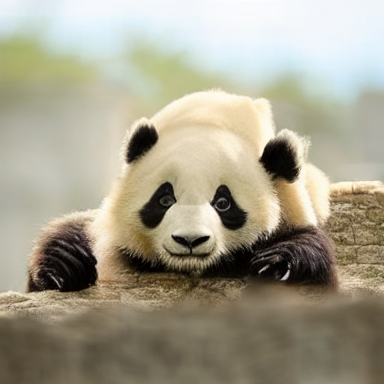}\\

      \includegraphics[width=3cm]{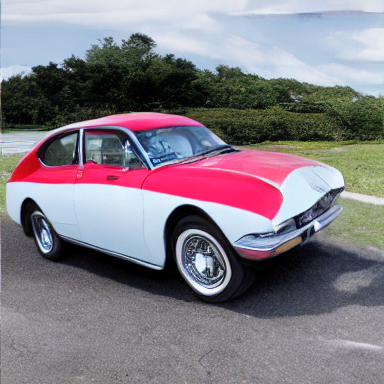} & \raisebox{0.5cm}{\rotatebox{90}{\parbox{2cm}{\centering a \textcolor{red}{pink} car}}} & \includegraphics[width=3cm]{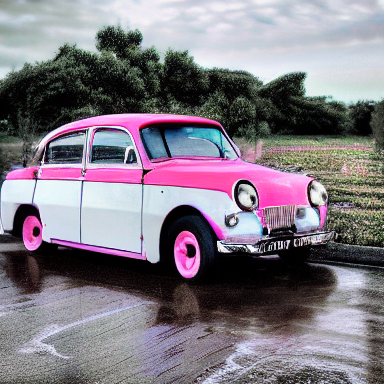} & \includegraphics[width=3cm]{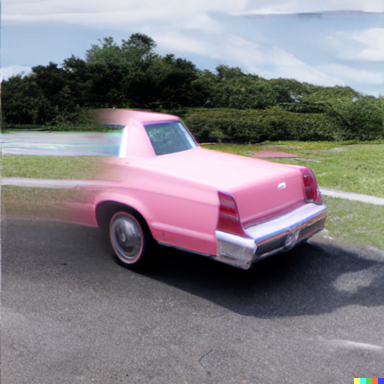} & \includegraphics[width=3cm]{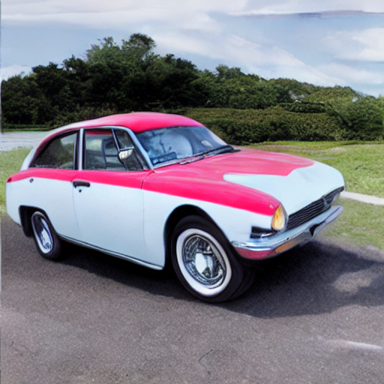} & \includegraphics[width=3cm]{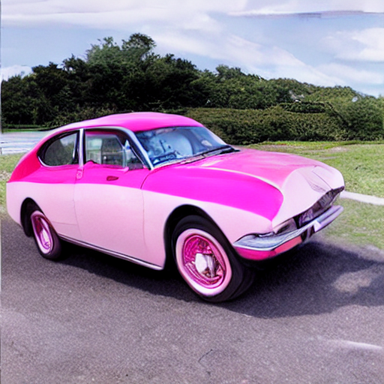} & \includegraphics[width=3cm]{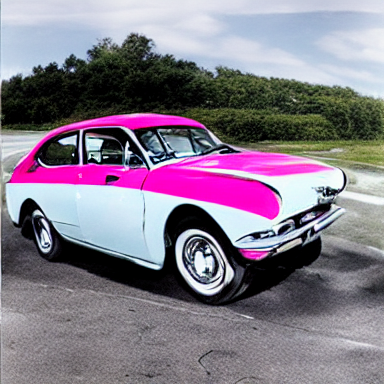}\\

      \includegraphics[width=3cm]{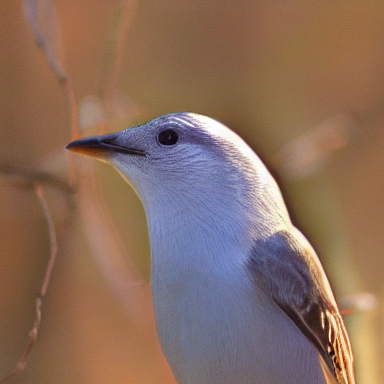} & \raisebox{0.5cm}{\rotatebox{90}{\parbox{2cm}{\centering a \textcolor{red}{parrot}}}} & \includegraphics[width=3cm]{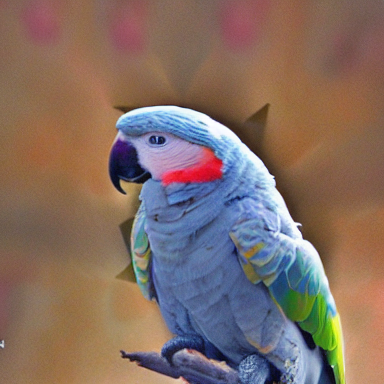} & \includegraphics[width=3cm]{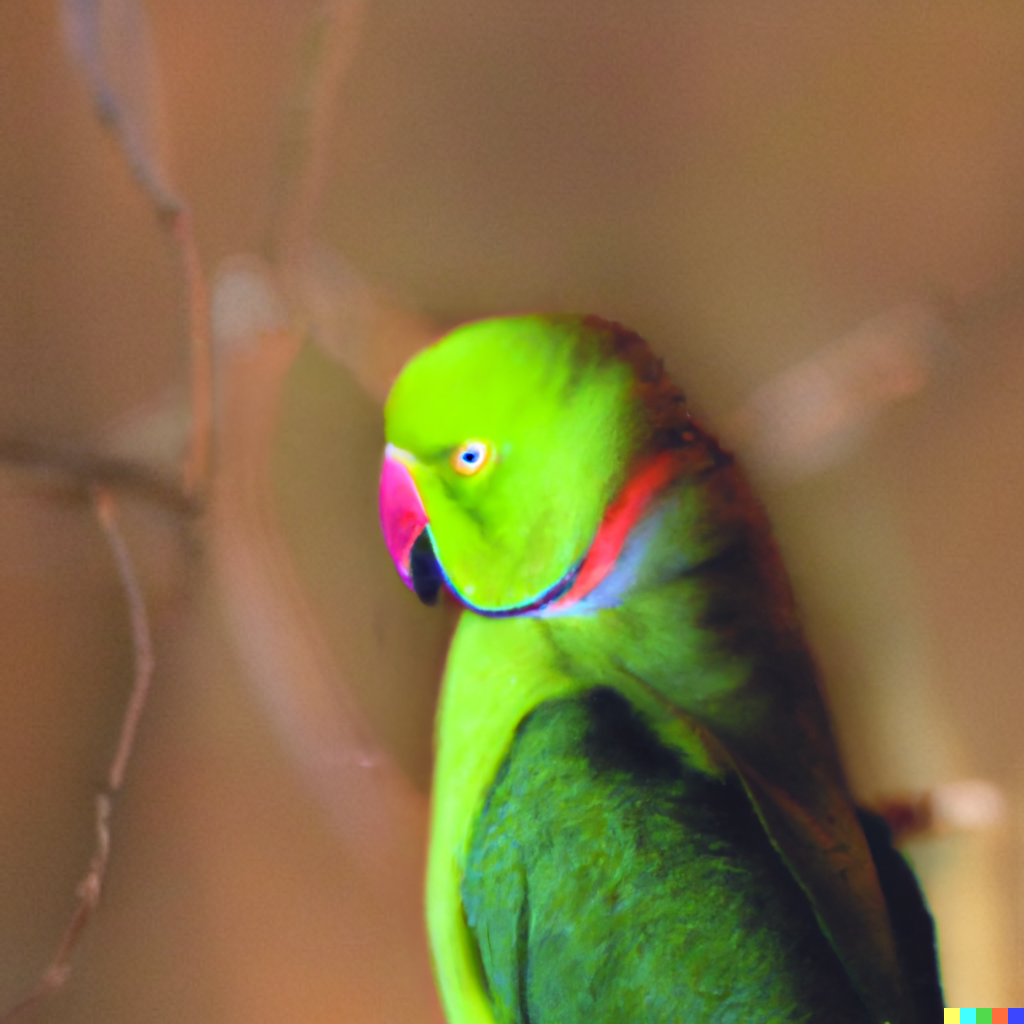} & \includegraphics[width=3cm]{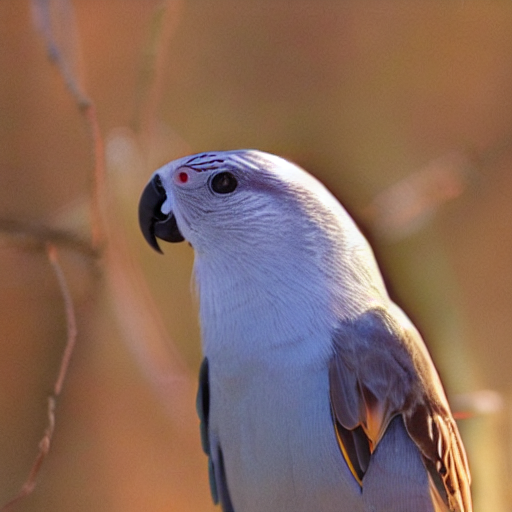} & \includegraphics[width=3cm]{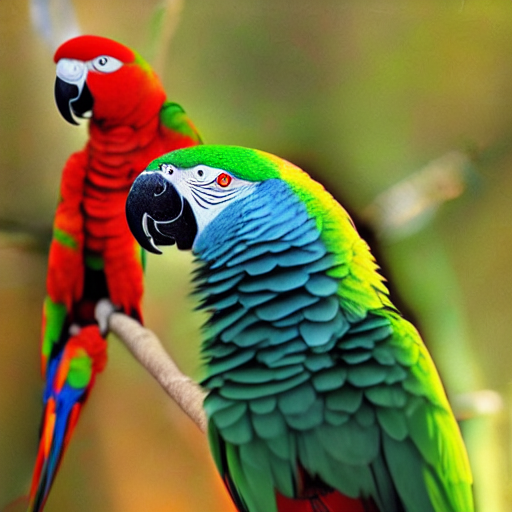} & \includegraphics[width=3cm]{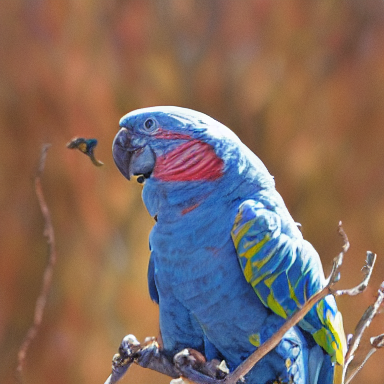}\\
      
      \includegraphics[width=3cm]{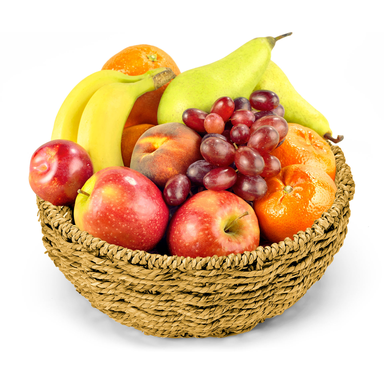} & \raisebox{0.5cm}{\rotatebox{90}{\parbox{2cm}{\centering a bowl of \cancel{fruits} \textcolor{red}{apples}}}} & \includegraphics[width=3cm]{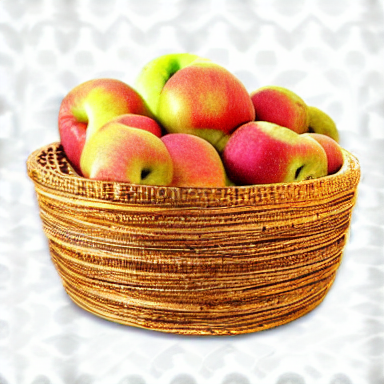} & \includegraphics[width=3cm]{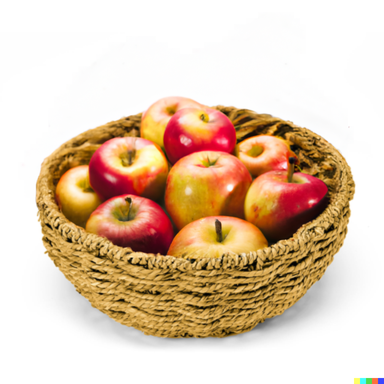} & \includegraphics[width=3cm]{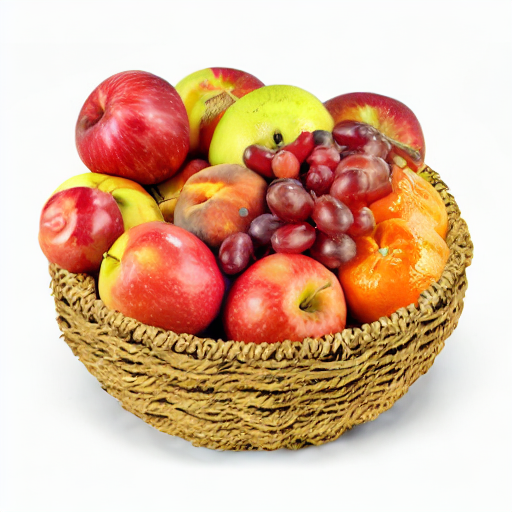} & \includegraphics[width=3cm]{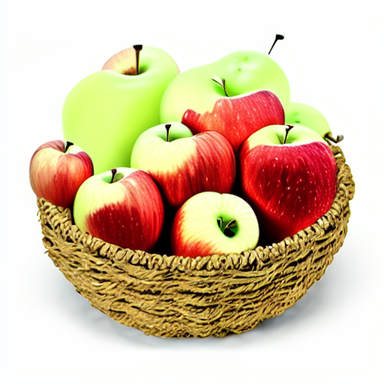} & \includegraphics[width=3cm]{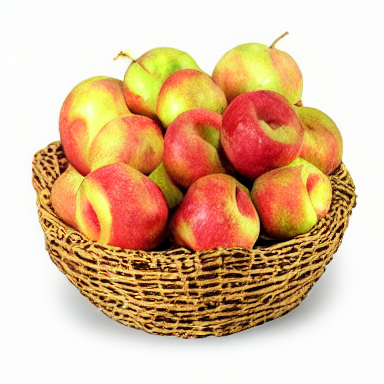}\\
      
      \includegraphics[width=3cm]{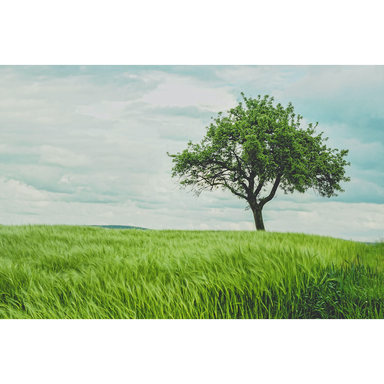} & \raisebox{0.5cm}{\rotatebox{90}{\parbox{2cm}{\centering an \textcolor{red}{autumn} tree}}} & \includegraphics[width=3cm]{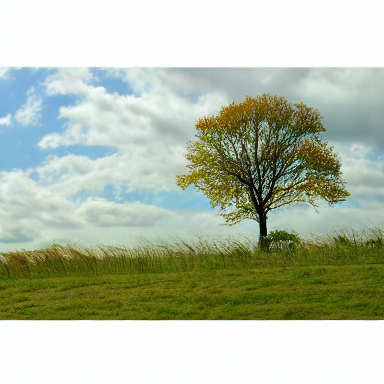} & \includegraphics[width=3cm]{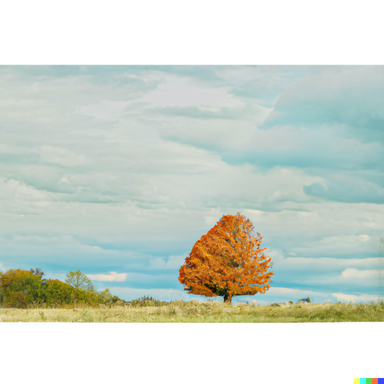} & \includegraphics[width=3cm]{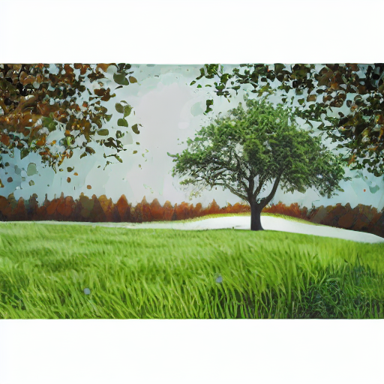} & \includegraphics[width=3cm]{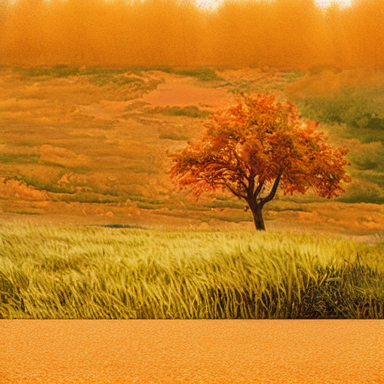} & \includegraphics[width=3cm]{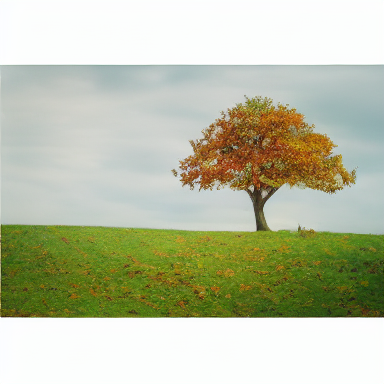}\\
      
      \includegraphics[width=3cm]{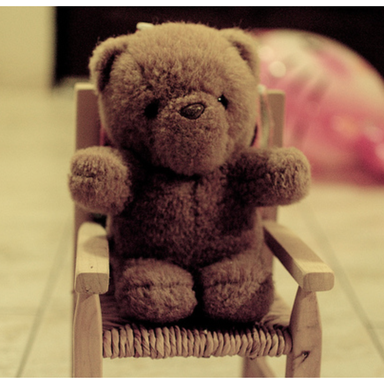} & \raisebox{0.5cm}{\rotatebox{90}{\parbox{2cm}{\centering a \textcolor{red}{dog}}}} & \includegraphics[width=3cm]{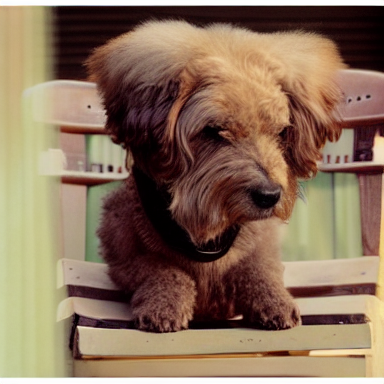} & \includegraphics[width=3cm]{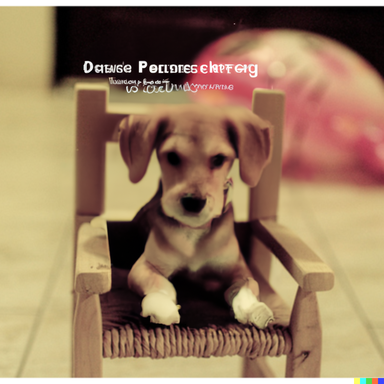} & \includegraphics[width=3cm]{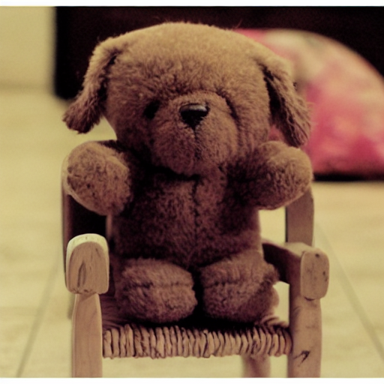} & \includegraphics[width=3cm]{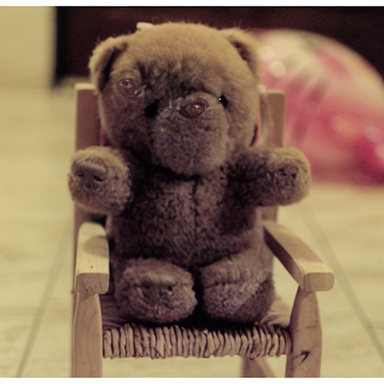} & \includegraphics[width=3cm]{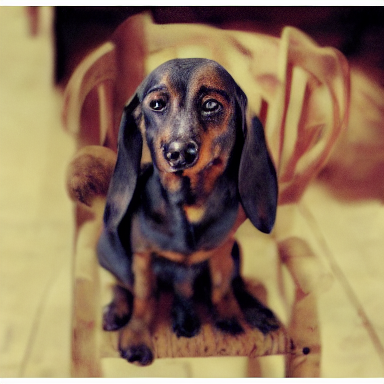}\\
      
      \includegraphics[width=3cm]{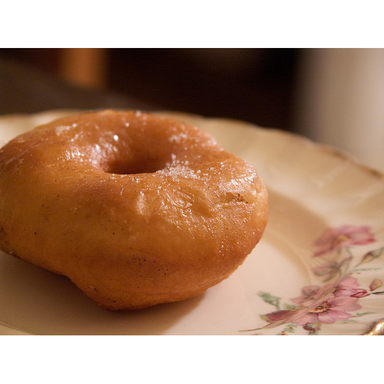} & \raisebox{0.5cm}{\rotatebox{90}{\parbox{2cm}{\centering \scriptsize{a doughnut \textcolor{red}{with\\ white chocolate and raspberry sauce}}}}} & \includegraphics[width=3cm]{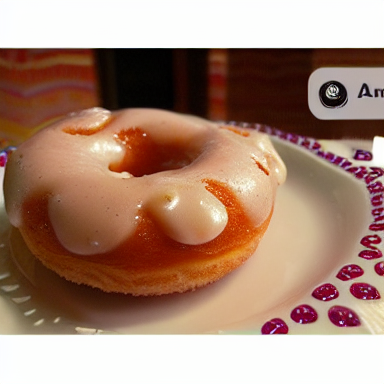} & \includegraphics[width=3cm]{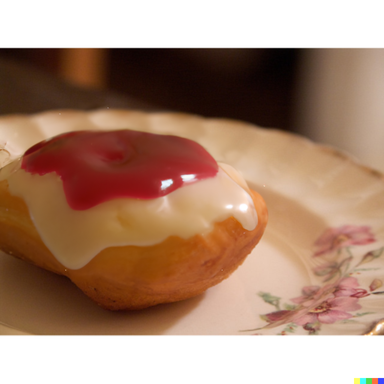} & \includegraphics[width=3cm]{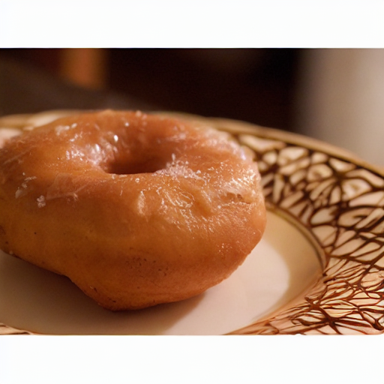} & \includegraphics[width=3cm]{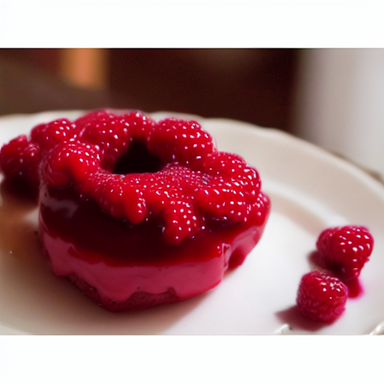} & \includegraphics[width=3cm]{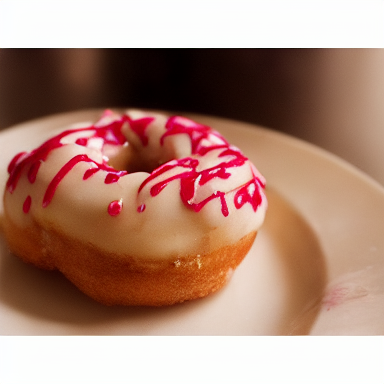}\\
    \end{tabular}%
  }
  \caption{Additional qualitative  results comparing our method against SDEdit~\cite{meng2022sdedit}, DALL-E 2~\cite{ramesh2022dalle}, DiffEdit~\cite{diffedit} and InstructPixtoPix~\cite{brooks2022instructpix2pix} using both generated and real images.}
  \label{fig:supp_qual_sota_comparison}
\end{figure*}

Figure~\ref{fig:supp_qual_sota_comparison} showcases additional qualitative comparisons between our method and prominent approaches, including SDEdit~\cite{meng2022sdedit}, DALL-E 2~\cite{ramesh2022dalle}, DiffEdit~\cite{diffedit}, and InstructPix2Pix~\cite{brooks2022instructpix2pix}. Our observations echo those discussed in the main paper. Notably, SDEdit~\cite{meng2022sdedit} grapples with the challenge of maintaining a balance between fidelity to the input image and adherence to the target prompt, as evident in examples like `a boat in the sea', `a bowl of apples', and `a pink car'. DALL-E 2~\cite{ramesh2022dalle}, functioning as an inpainting method reliant on masks, tends to discard content within the masked area while preserving the inverse mask area. This often leads to mismatches between input and edited content, as seen in the positions of `a leopard', `a panda', `an autumn tree', and the quantity of `apples'. Additionally, it encounters difficulty in seamlessly blending with the rest of the image, exemplified by the case of pink car'. DiffEdit's sensitivity to detected masks, dependent on parameters and the employed image generation model, results in occasional failures in accurate mask detection (a leopard', a panda', a bowl of apples') or the selection of completely incorrect areas (`doughnut', `autumn tree'). InstructPix2Pix may generate non-realistic images (`a panda', `a leopard'), face translation issues (e.g., `teddy bear translated into a dog'), impact the entire image with the target prompt (`a parrot', `autumn tree', `a pink car'), or struggle with multiple simultaneous changes (e.g., `doughnut with raspberry and white chocolate sauce'). Despite not using masks at inference like DALL-E 2 and DiffEdit and not being trained on a dataset with target images like InstructPix2Pix, our method achieves more successful translations with high fidelity to the target prompt and input image, accompanied by minimal undesired changes.

\section{User Study}

As described in the main paper, we executed a user study adhering to established procedures on Microworkers. A total of 540 pairs were presented to users, each consisting of input images, target prompts, and manipulation outcomes generated by both our proposed method and a baseline.
Each pair underwent evaluation by 10 distinct participants, tasked with identifying the more effective manipulation in terms of fidelity to the prompt and input image. This process yielded a comprehensive dataset of 5.4K responses. The outcomes of this survey are detailed in Table~\ref{tab:quantitative-comparison} of the main paper. The results consistently demonstrate a preference for our proposed method over the baseline.

\section{Integrating DiffEdit into Our Framework}

In Figure~\ref{fig:diffours}, we provide additional qualitative comparisons between our method and DiffEdit~\cite{diffedit}. The first column shows the input image, and the second and third columns display DiffEdit and our results, respectively. As DiffEdit is exclusively utilised at inference time, we seamlessly incorporate it into our method, presenting the combined outcomes in the last column. Identical parameters are employed for computations in both DiffEdit and DiffEdit$+$Ours. DiffEdit utilises Stable Diffusion's checkpoint v1.4, the same pretrained model used for fine-tuning with our approach.

\begin{figure}[!t]
  \centering
  \resizebox{\linewidth}{!}{%
    \begin{tabular}{ccccc}
      { Input} && { DiffEdit} & {Ours} & {DiffEdit $+$ Ours} \\
     
      \includegraphics[width=3cm]{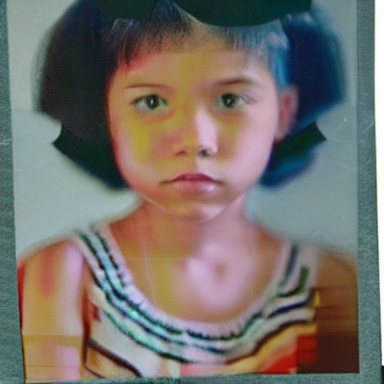} & \raisebox{0.5cm}{\rotatebox{90}{\parbox{2cm}{\centering a girl \textcolor{orange}{wearing\\ a hat}}}} & \includegraphics[width=3cm]{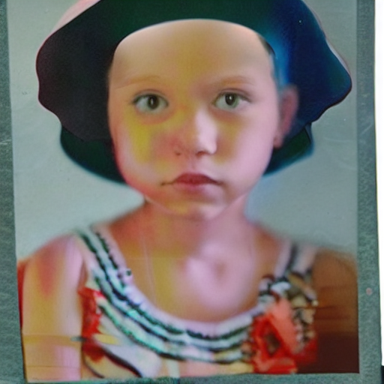} & \includegraphics[width=3cm]{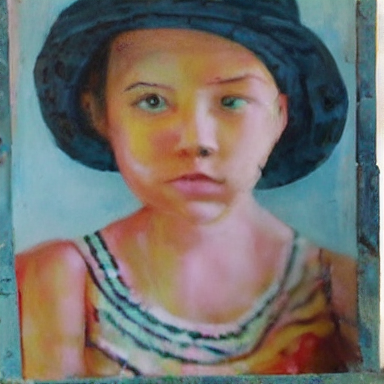} & \includegraphics[width=3cm]{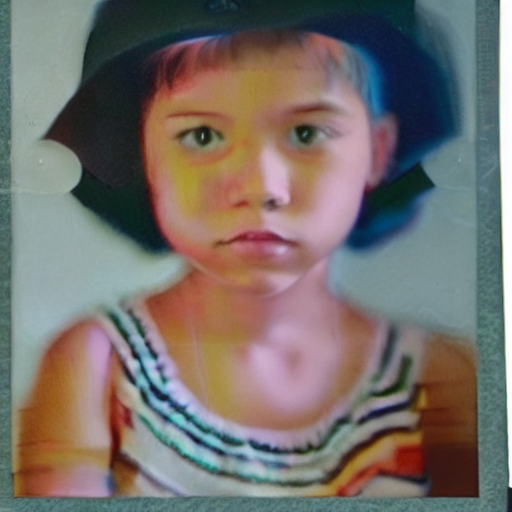} \\

       \includegraphics[width=3cm]{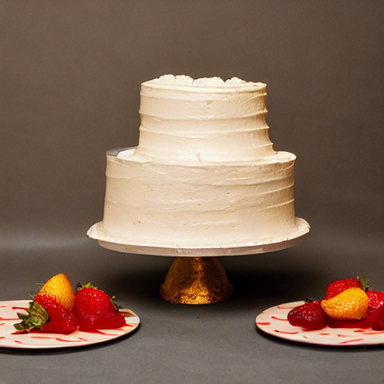} & \raisebox{0.5cm}{\rotatebox{90}{\parbox{2cm}{\centering a \textcolor{orange}{three-tier}\\  cake}}} & \includegraphics[width=3cm]{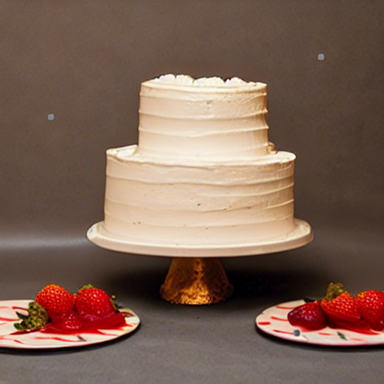} & \includegraphics[width=3cm]{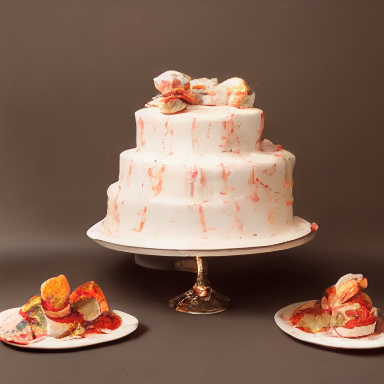} & \includegraphics[width=3cm]{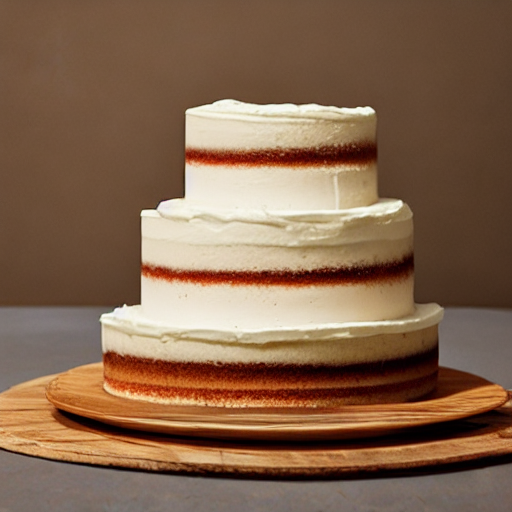}
      \\

       \includegraphics[width=3cm]{figs/supp_diffedit_ours/0002.png} & \raisebox{0.5cm}{\rotatebox{90}{\parbox{2cm}{\centering a \textcolor{orange}{strawberry}\\  cake}}} & \includegraphics[width=3cm]{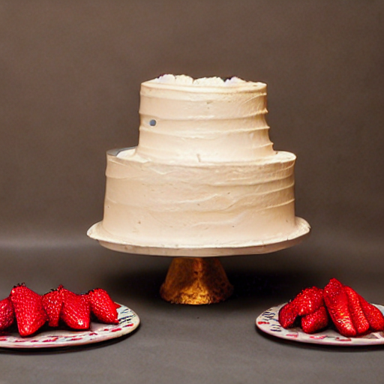} & \includegraphics[width=3cm]{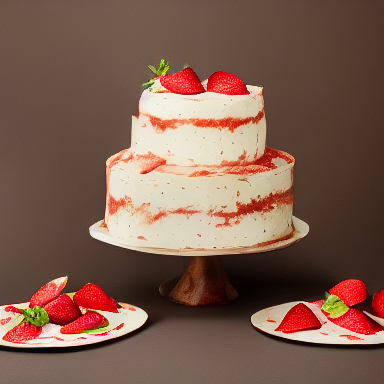} & \includegraphics[width=3cm]{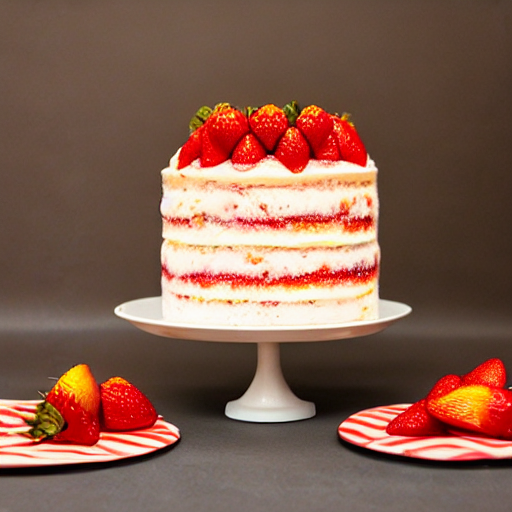}
      \\

      \includegraphics[width=3cm]{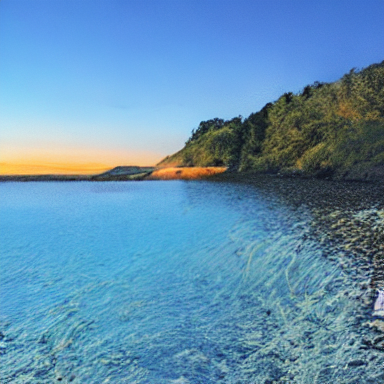} & \raisebox{0.5cm}{\rotatebox{90}{\parbox{2cm}{\centering a \textcolor{orange}{moon in the} sky}}} & \includegraphics[width=3cm]{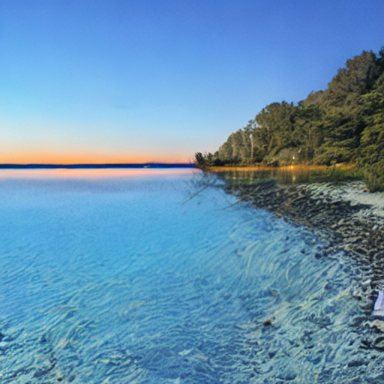} & \includegraphics[width=3cm]{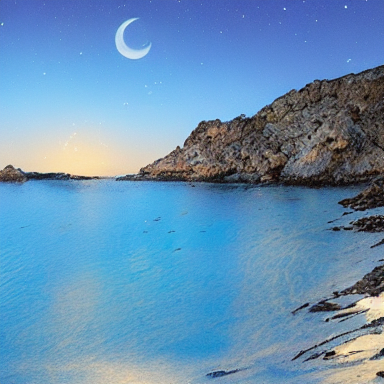} & \includegraphics[width=3cm]{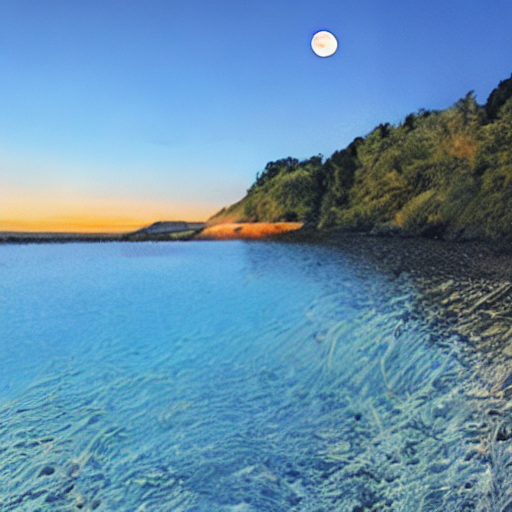} \\

      \includegraphics[width=3cm]{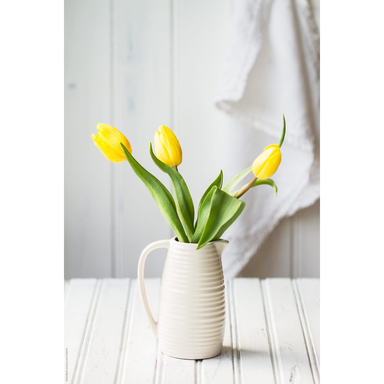} & \raisebox{0.5cm}{\rotatebox{90}{\parbox{2cm}{\centering \textcolor{orange}{lavenders} \cancel{tulips} in \\ a \textcolor{orange}{glass} vase}}} & \includegraphics[width=3cm]{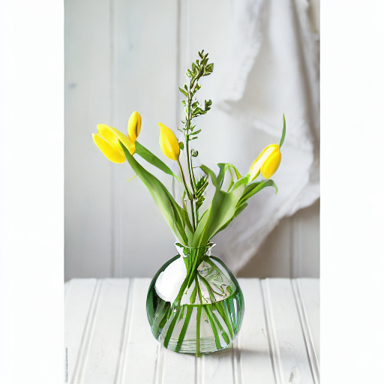} & \includegraphics[width=3cm]{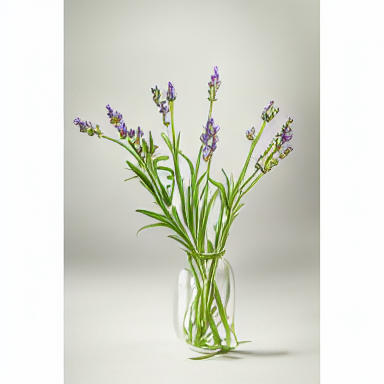} & \includegraphics[width=3cm]{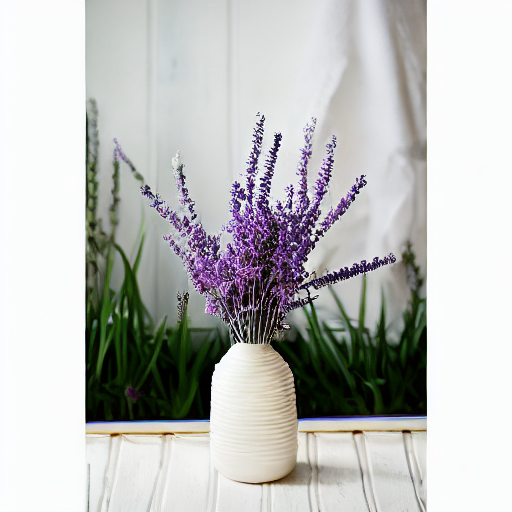} \\
      
      \includegraphics[width=3cm]{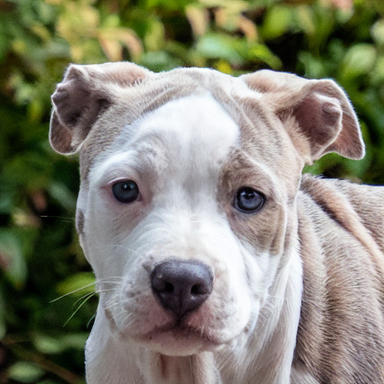} & \raisebox{0.5cm}{\rotatebox{90}{\parbox{2cm}{\centering a \textcolor{orange}{yorkshire terrier}}}} & \includegraphics[width=3cm]{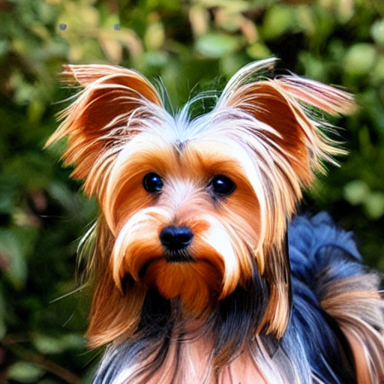} & \includegraphics[width=3cm]{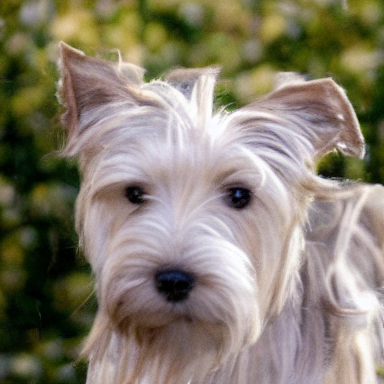} & \includegraphics[width=3cm]{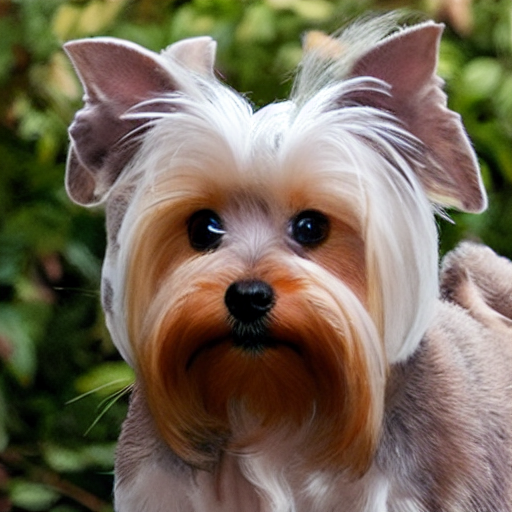} \\

    \end{tabular}%
  }
  \caption{Qualitative comparison of DiffEdit, our method and their combination.}
  \label{fig:diffours}
\end{figure}

When using DiffEdit in conjunction with our method, we observe improved mask detection. For example, in `a girl wearing a hat', DiffEdit alters the girl's face while adding a hat. Upon integration into our method at inference, the face remains unaltered while incorporating the hat. Our method alone achieves a successful translation with minimal undesired modifications in the face area, and this is further mitigated with the integration of DiffEdit. A similar scenario is evident in "a moon in the sky," where DiffEdit manipulates an unrelated area on the shores. Integrated into our method, it produces a successful translation while preserving unrelated areas effectively. Once again, our method alone, while placing the moon in the desired location, introduces some undesired alterations, which are minimized through the integration of DiffEdit. In `a strawberry cake', DiffEdit inaccurately manipulates the plates rather than the cake. While our method achieves a successful translation with minimal undesired changes, integration with DiffEdit further prevents these changes, preserving all parts of the image perfectly. These results highlight that our fine-tuning strategy enhances the model's ability to detect editing masks compared to the baseline.

Consistent with our earlier observations, while our method enhances the accuracy of mask detection in DiffEdit, it remains sensitive to the detected masks and corresponding parameters. An example is seen in `lavenders', where integrating DiffEdit into our framework leads to undesired manipulations in the background and fails to successfully translate the vase into a glass one although it preserves some details better. Despite DiffEdit detecting a relatively accurate mask in this case, it struggles to translate tulips into lavenders successfully. In summary, while integrating DiffEdit often improves our method, particularly in preserving the background, its performance is still influenced by parameter sensitivity in mask detection. Further refinement of these parameters could enhance the overall results.
